# Supplementary material for: GLane3D : Detecting Lanes with Graph of 3D Keypoints
Source: arXiv:2503.23882 source file (2025-03-31)
Supplement: Supplementary file 1 [file appendix.tex]

\begin{table*}
     \begin{tabular}{ c | l |  l | c |  c |  c c | c c} 
    \Xhline{1.3pt}
     Dist. & Methods & Backbone & F1-Score(\%)\uparrow & AP(\%)\uparrow &\begin{tabular}{@{}c@{}}X-error \\  near(m) \downarrow  \end{tabular}  & \begin{tabular}{@{}c@{}}X-error \\  far(m) \downarrow  \end{tabular}   & \begin{tabular}{@{}c@{}}Z-error \\  near(m) \downarrow \end{tabular} & \begin{tabular}{@{}c@{}}Z-error \\  far(m) \downarrow  \end{tabular}  \\ [0.5ex] 
    \hhline{=========}
    
     \parbox[t]{2mm}{\multirow{6}{*}{\rotatebox[origin=c]{90}{\textit{Balanced Scene}}}} 
     & PersFormer\cite{chen2022persformer} & EffNet-B7 & 92.9 & -  & 0.054 & 0.356 & 0.010  & 0.234  \\
     & BEVLaneDet \cite{wang2023bev} & ResNet-34 & 96.9 & - & \textbf{0.016} & \textbf{0.242} & 0.020  & 0.216   \\
     & LaneCPP \cite{pittner2024lanecpp} &  EffNet-B7 & \underline{97.4} & \textbf{99.5} & 0.030 & 0.277 & 0.011  & \textbf{0.206}  \\
     & LATR \cite{luo2023latr}& ResNet-50 & 96.8 & 97.9 & 0.022 & 0.253 & \textbf{0.007}  & \textbf{0.202} \\
     & DV-3DLane \cite{luo2024dv}& ResNet-50 & 96.4 & 97.6 & 0.046 & 0.299 & 0.016  & \underline{0.213} \\
    \cline{2-8} & \rowcolor{lightgray} BEVLaneG (Ours) & ResNet-50 & \textbf{98.1} & \underline{98.8} & \underline{0.021} & \textbf{0.250} & \underline{0.007}  & 0.213 \\

    \Xhline{1.3pt}

    \parbox[t]{2mm}{\multirow{6}{*}{\rotatebox[origin=c]{90}{\textit{Rare Scene}}}} 
     & PersFormer\cite{chen2022persformer} & EffNet-B7 & 87.5 & -  & 0.107 & 0.782 & 0.024  & 0.602  \\
     & BEVLaneDet \cite{wang2023bev} & ResNet-34 & \underline{97.6} & - & \textbf{0.031} & \textbf{0.594} & 0.040  & 0.556   \\
     & LaneCPP \cite{pittner2024lanecpp} &  EffNet-B7 & 96.2 & \underline{98.6} & 0.073 & 0.651 & \underline{0.023}  & \underline{0.543}  \\
     & LATR \cite{luo2023latr}& ResNet-50 & 96.1 & 97.3 & 0.050 & \underline{0.600} & \textbf{0.015}  & \textbf{0.532} \\
     & DV-3DLane \cite{luo2024dv}& ResNet-50 & 95.5 & 97.2 & 0.071 & 0.664 & 0.025  & 0.568 \\
    \cline{2-8} & \rowcolor{lightgray} BEVLaneG (Ours) & ResNet-50 & \textbf{98.4} & \textbf{99.1} & \underline{0.044} & 0.621 & 0.023  & 0.566 \\
    
    \Xhline{1.3pt}

   \parbox[t]{2mm}{\multirow{6}{*}{\rotatebox[origin=c]{90}{\textit{Visual Variations}}}} 
     & PersFormer\cite{chen2022persformer} & EffNet-B7 & 89.6 & -  & 0.074 & 0.430 & \textbf{0.015}  & 0.266  \\
     & BEVLaneDet \cite{wang2023bev} & ResNet-34 & \underline{95.0} & - & \textbf{0.027} & \underline{0.320} & 0.031  & 0.256   \\
     & LaneCPP \cite{pittner2024lanecpp} &  EffNet-B7 & 90.4 & 93.7 & 0.054 & 0.327 & 0.020  & \textbf{0.222}  \\
     & LATR \cite{luo2023latr}& ResNet-50 & \textbf{95.1} & \textbf{96.6} & 0.045 & \textbf{0.315} & \underline{0.016}  & \underline{0.228} \\
     & DV-3DLane \cite{luo2024dv}& ResNet-50 & 91.3 & 93.4 & 0.095 & 0.417 & 0.040  & 0.320 \\
    \cline{2-8} & \rowcolor{lightgray} BEVLaneG (Ours) & ResNet-50 & 92.7 & \underline{94.8} & 0.046 & 0.364 & 0.020  & 0.317 \\
    \Xhline{1.3pt}

    \end{tabular}
   \caption{}
   \label{tab:apollo}
\end{table*}
